# Supplementary material for: Multiple imputation with missing data indicators
Source: arXiv:2103.02033 ancillary file (2021-03-02)
Supplement: Supplementary file 1 [file supplemental_material.pdf]

# Supplemental Material to “Multiple imputation with missing data indicators”

Lauren J Beesley, Irina Bondarenko, Michael R Elliott,  
Allison W Kurian, Steven J Katz, Jeremy M G Taylor

## A Additional simulation results

Figure A.1: Bias in estimation of missingness model parameters across 200 simulated datasets using data imputed using the SRMI-Exact method

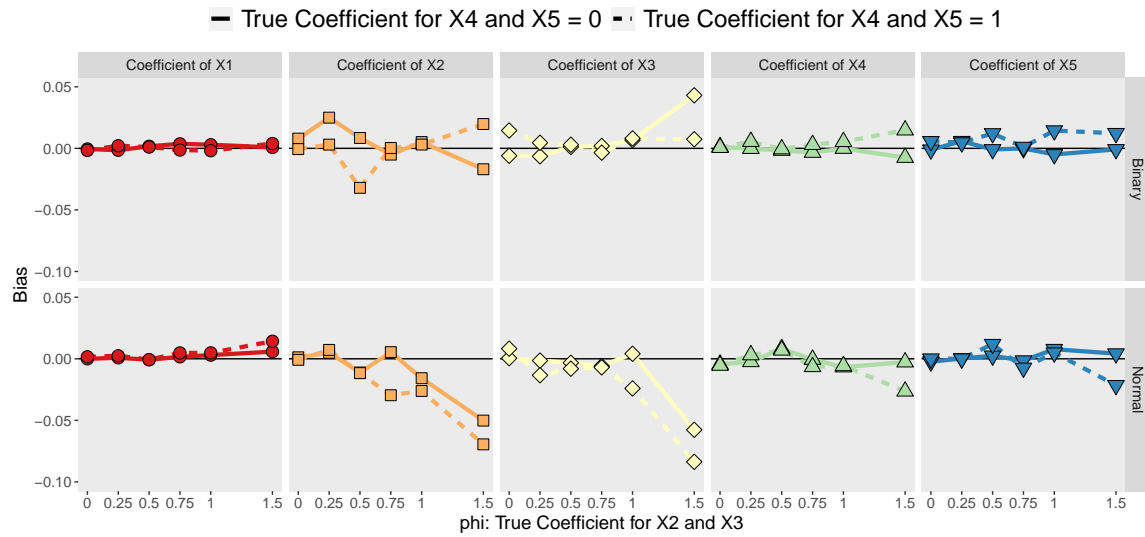

Figure A.2: Coverage of 95% confidence intervals for mean of  $X_1$  across 200 simulated datasets after applying various imputation strategies<sup>1</sup>

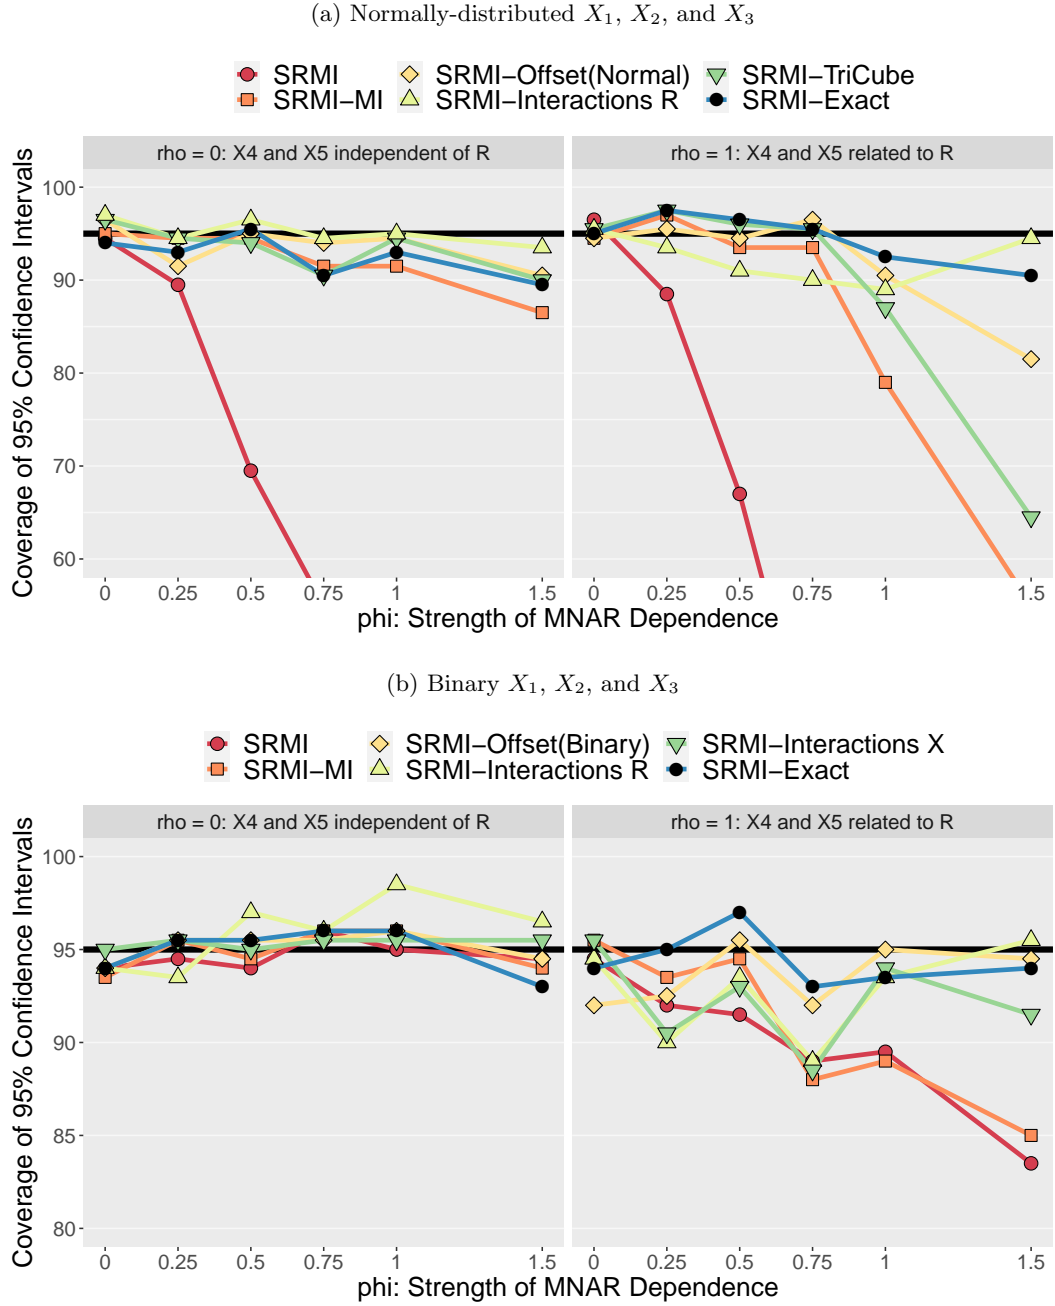

<sup>1</sup> Results shown for  $M = 10$  imputed datasets.

Figure A.3: Bias for regression of  $X_1|X_2, X_3, X_4, X_5$  across 200 simulated datasets after applying various imputation strategies<sup>1</sup>

(a) Linear regression and normally-distributed  $X_1, X_2$ , and  $X_3$

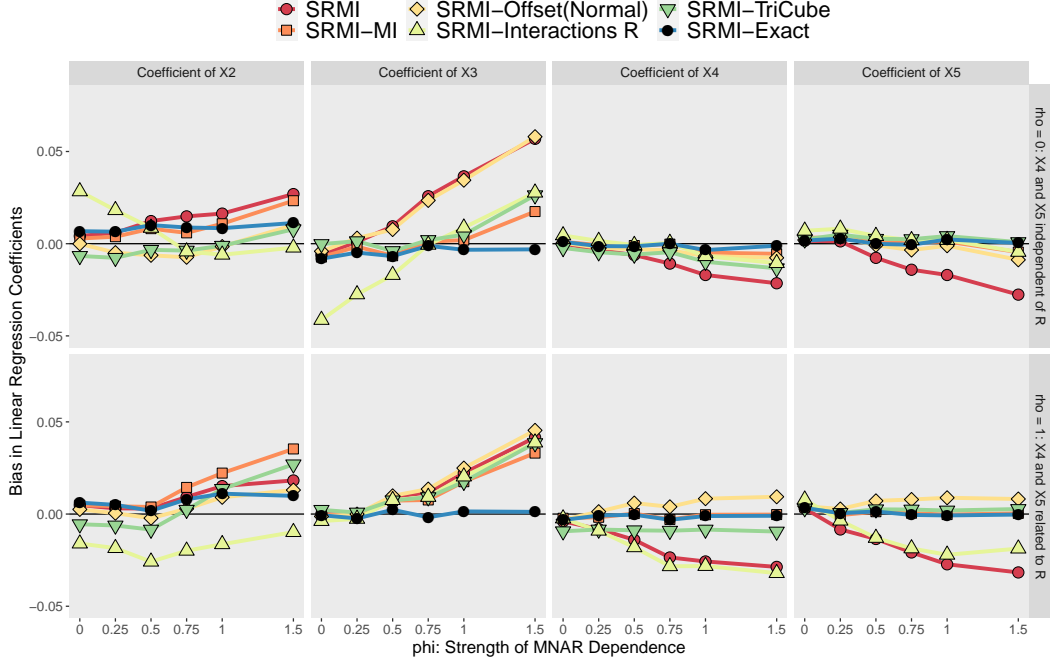

(b) Logistic regression and binary  $X_1, X_2$ , and  $X_3$

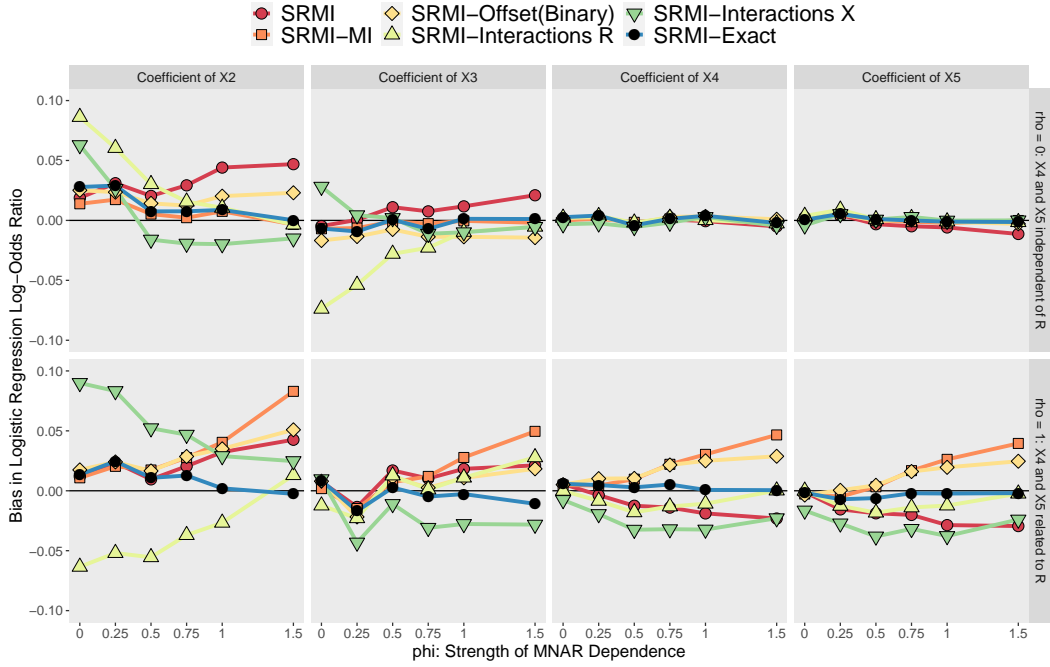

<sup>1</sup> Results shown for  $M = 10$  imputed datasets.

Figure A.4: Relative variances for regression of  $X_1|X_2, X_3, X_4, X_5$  across 200 simulated datasets after applying various imputation strategies, relative to analysis of full data without missingness<sup>1</sup>

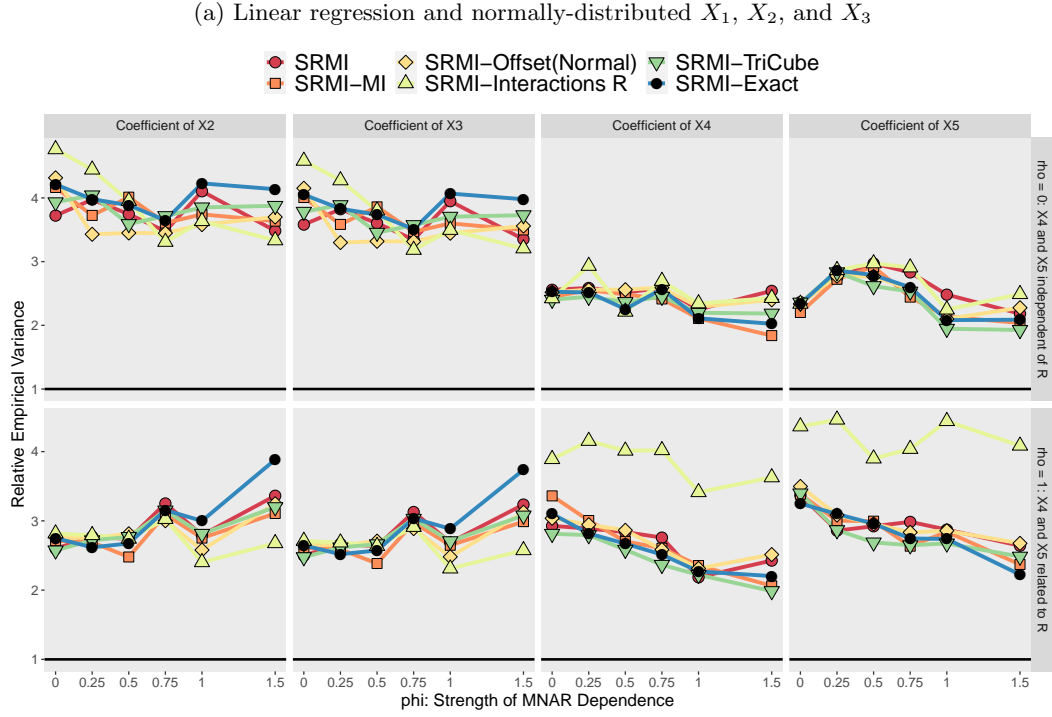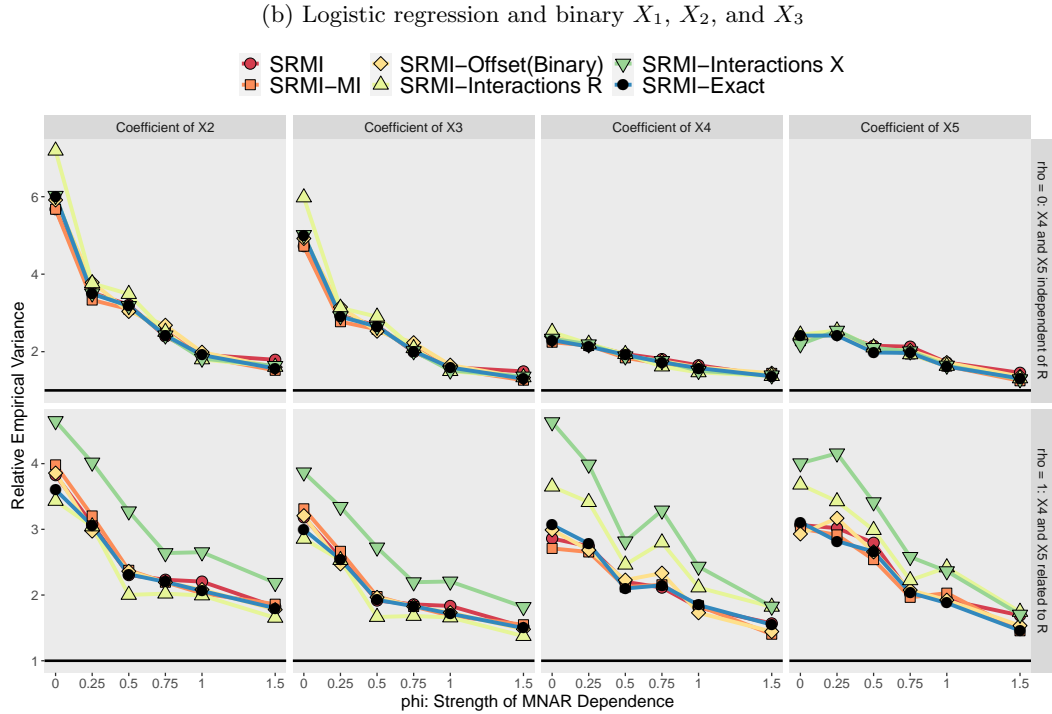

<sup>1</sup> Results shown for  $M = 10$  imputed datasets.

## B Simulation Study: imputation of rare binary variables

In the course of our exploration, we observed that chained equations multiple imputation can produce bias in estimating the mean of  $X_1$  for rare binary  $X_1$  (e.g. prevalence  $<5\%$ ) even under simple MAR settings. We conducted a set of simulations in which binary  $X_1$ - $X_5$  were generated under a multivariate normal distribution as described previously but where covariates  $X_1$ ,  $X_2$ , and  $X_3$  were dichotomized to take the value 1 if the drawn value was above the 99th standard normal quantile. This resulted in a marginal prevalence of about 1% for each of  $X_1$ ,  $X_2$ , and  $X_3$ . Missing values were then imputed using SRMI and SRMI-MI. For each approach, we consider two variations. In the first, missing values for each  $X_j$  were imputed using the ‘logreg’ imputation function in *mice*. This implements imputation assuming a logistic regression model for  $X_j$ , using a multivariate normal approximation to draw imputation model parameters and implementing a data augmentation strategy prior to imputation (1). We also propose an alternative imputation strategy where parameters are drawn by fitting a logistic regression model to a bootstrap sample of the imputed data, stratified by  $X_j$ . By stratifying the bootstrap sampling by  $X_j$ , we ensure that no bootstrap sample will have no 1’s. By relying on point estimates from a bootstrap sample, the resulting draws do not rely on good properties of variance estimation under low outcome prevalence (unlike the strategy used by ‘logreg’). Our stratified bootstrap results did not incorporate the data augmentation pre-processing step implemented by ‘logreg.’ Using these two imputation variations, we implemented the methods in SRMI and SRMI-MI corresponding to excluding and including the missingness indicators in the imputation models, respectively. We then calculated the mean of  $X_1$  and the empirical variance for the mean of  $X_1$  across the 200 simulated datasets.

**Figure B.1a** shows the bias in estimating the mean of  $X_1$  for imputation of rare binary covariates. Imputation using the ‘logreg’ function in the R package *mice* resulted in non-negligible bias. In contrast, the proposed stratified bootstrap imputation approach resulted in little bias. Little difference between the SRMI and SRMI-MI imputation strategies were seen here.

One concern is that the stratified bootstrap sampling used to obtain parameter draws may result in empirical variances that are too small. **Figure B.1b** shows the relative empirical variance estimates. In settings where  $\rho$  was 1 (so continuous  $X_4$  and  $X_5$  were in the true missingness model), the stratified bootstrap method did result in smaller standard errors than the other method. However, the corresponding 95% confidence intervals had nominal coverage, indicating that the empirical variances for the logreg imputation were inflated.

Figure B.1: Estimated mean of  $X_1$  and relative variance across 200 simulated datasets after applying various imputation strategies for rare binary  $X_1$ ,  $X_2$ , and  $X_3$

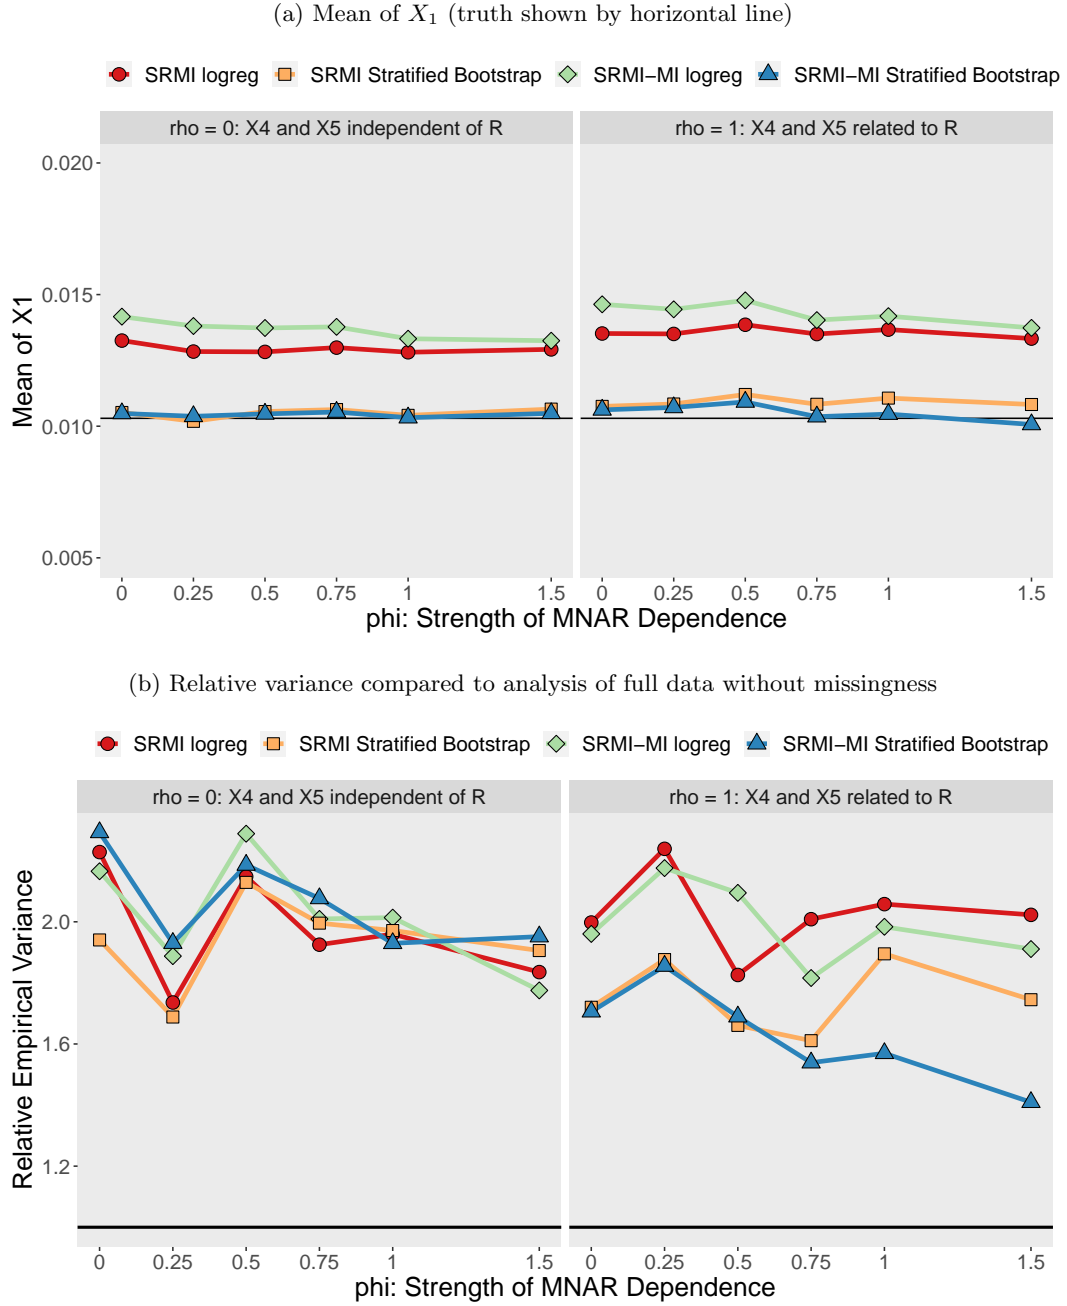

<sup>1</sup> Results shown for  $M = 10$  imputed datasets.

## C Additional results for breast cancer dataset

Table C.1: Summary statistics for the variables in the dataset. Sample size = 5080.

| Variable                          | Category                      | number of people | percent |
|-----------------------------------|-------------------------------|------------------|---------|
| BRCA1/2                           | Negative/VUS                  | 1330             | 26.2    |
|                                   | Positive                      | 65               | 1.3     |
|                                   | Missing                       | 3685             | 72.5    |
| Age                               | <40                           | 154              | 3.0     |
|                                   | 40-65                         | 3051             | 60.1    |
|                                   | >65                           | 1820             | 35.8    |
|                                   | Missing                       | 55               | 1.1     |
| Race                              | White                         | 2716             | 53.5    |
|                                   | Black                         | 930              | 18.3    |
|                                   | Hispanic                      | 905              | 17.8    |
|                                   | Asian, Pacific Island, Others | 458              | 9.0     |
|                                   | Missing                       | 71               | 1.4     |
| SEER site                         | Los Angeles                   | 2486             | 48.9    |
|                                   | Georgia                       | 2594             | 51.1    |
| Family history of cancer          | No                            | 3388             | 66.7    |
|                                   | Yes                           | 1157             | 22.8    |
|                                   | Missing                       | 535              | 10.5    |
| Jewish ancestry                   | No                            | 4621             | 91.0    |
|                                   | Yes                           | 207              | 4.1     |
|                                   | Missing                       | 252              | 5.0     |
| Relative with known gene mutation | No                            | 3919             | 77.1    |
|                                   | Yes                           | 94               | 1.9     |
|                                   | Missing                       | 1067             | 21.0    |
| Bilateral cancer                  | No                            | 4825             | 95.0    |
|                                   | Yes                           | 255              | 5.0     |
| Clinical T stage                  | T0                            | 855              | 16.8    |
|                                   | T1                            | 3065             | 60.3    |
|                                   | T2                            | 1128             | 22.2    |
|                                   | Missing                       | 32               | 0.6     |
| Tumor grade                       | 1                             | 1193             | 23.5    |
|                                   | 2                             | 2255             | 44.4    |
|                                   | 3                             | 1439             | 28.3    |
|                                   | Missing                       | 193              | 3.8     |
| Lymph Node invasion               | No                            | 4173             | 82.1    |
|                                   | Yes                           | 841              | 16.6    |
|                                   | Missing                       | 66               | 1.3     |
| ER status                         | Negative                      | 627              | 12.3    |
|                                   | Positive                      | 4327             | 85.2    |
|                                   | Missing                       | 126              | 2.5     |
| PR status                         | Negative                      | 1066             | 21.0    |
|                                   | Positive                      | 3761             | 74.0    |
|                                   | Missing                       | 253              | 5.0     |
| HER2 status                       | Negative                      | 625              | 12.3    |
|                                   | Positive/Borderline           | 3535             | 69.6    |
|                                   | Missing                       | 920              | 18.1    |

Table C.2: Odds ratios (95% CI) for the probability that BRCA1/2 test result is missing. Analysis based on the n= 2863 women who have complete data on all the listed risk factors.

| Variable                    | Category | Odds Ratio (95% CI) |
|-----------------------------|----------|---------------------|
| Age/5 years                 |          | 0.89 (0.88,0.90)    |
| Race/ethnicity (ref=White)  | Black    | 0.53 (0.40,0.71)    |
|                             | Hispanic | 0.33 (0.23,0.47)    |
|                             | Other    | 0.59 (0.40,0.88)    |
| SEER site (ref=Los Angeles) | Georgia  | 1.69 (1.32,2.16)    |
| Family history of cancer    |          | 3.72 (2.96,4.66)    |
| Jewish ancestry             |          | 6.03 (3.94,9.23)    |
| Relative with gene mutation |          | 1.99 (1.04,3.79)    |
| Bilateral cancer            |          | 3.84 (2.61,5.66)    |
| Clinical T stage (ref=T0)   | T1       | 1.45 (0.75,2.80)    |
|                             | T2       | 1.48 (0.75,2.91)    |
| Tumor grade (Ref=1)         | 2        | 0.97 (0.77,1.23)    |
|                             | 3+       | 1.20 (0.89,1.62)    |
| Lymph node invasion         |          | 1.08 (0.85,1.38)    |
| ER                          | Positive | 0.69 (0.47,1.01)    |
| PR                          | Positive | 0.88 (0.64,1.21)    |
| HER2                        | Positive | 0.72 (0.54,0.96)    |

Table C.3: Odds ratios (95% CI) for the probability that a woman has a BRCA1/2 pathogenic variant. Analysis of the complete cases is based on the n= 874 woman who have BRCA1/2 test results. Analyses in the SRMI columns are based on data from 5080 women.

| Variable                    | Category | Complete Cases     | SRMI               | SRMI-MI            | SRMI-Offset        |
|-----------------------------|----------|--------------------|--------------------|--------------------|--------------------|
| Age/5 years                 |          | 0.96 (0.92,0.99)   | 0.95 (0.92,0.99)   | 0.95 (0.92,0.98)   | 0.95 (0.92,0.97)   |
| Race/ethnicity (ref=White)  | Black    | 0.94 (0.37,2.41)   | 0.70 (0.35,1.37)   | 0.66 (0.32,1.37)   | 0.71 (0.36,1.40)   |
|                             | Hispanic | 0.16 (0.03,1.03)   | 0.62 (0.27,1.43)   | 0.57 (0.26,1.22)   | 0.61 (0.24,1.56)   |
|                             | Other    | 0.59 (0.10,3.36)   | 0.20 (0.02,1.63)   | 0.16 (0.02,1.30)   | 0.27 (0.04,1.88)   |
| SEER site (ref=Los Angeles) | Georgia  | 0.74 (0.32,1.73)   | 0.74 (0.42,1.31)   | 0.77 (0.40,1.50)   | 0.87 (0.45,1.71)   |
| Family history of cancer    |          | 2.69 (1.29,5.60)   | 2.00 (1.00,3.97)   | 2.34 (1.01,5.38)   | 2.18 (1.04,4.56)   |
| Jewish ancestry             |          | 2.58 (0.89,7.44)   | 1.35 (0.48,3.80)   | 1.21 (0.36,4.09)   | 1.85 (0.63,5.45)   |
| Relative with gene mutation |          | 12.59 (5.18,30.62) | 13.95 (6.48,30.05) | 13.36 (5.60,31.85) | 13.53 (7.07,25.87) |
| Bilateral cancer            |          | 1.73 (0.63,4.75)   | 1.39 (0.48,3.99)   | 1.36 (0.51,3.61)   | 1.58 (0.56,4.44)   |
| Clinical T stage (ref=T0)   | T1       | 1.94 (0.12,31.99)  | 2.91 (0.92,9.18)   | 2.32 (0.68,7.95)   | 2.31 (0.88,6.06)   |
|                             | T2       | 1.06 (0.06,18.93)  | 1.65 (0.52,5.30)   | 1.50 (0.42,5.34)   | 1.29 (0.44,3.79)   |
| Tumor grade (Ref=1)         | 2        | 2.57 (0.88,7.53)   | 3.11 (0.99,9.81)   | 2.71 (0.90,8.21)   | 3.33 (1.19,9.35)   |
|                             | 3+       | 2.38 (0.69,8.24)   | 4.70 (1.19,18.49)  | 3.60 (1.06,12.23)  | 4.49 (1.32,15.22)  |
| Lymph node invasion         |          | 2.05 (0.92,4.56)   | 1.79 (1.03,3.11)   | 1.99 (0.98,4.07)   | 1.99 (1.03,3.85)   |
| ER                          | Positive | 0.67 (0.21,2.17)   | 1.01 (0.44,2.31)   | 0.90 (0.39,2.08)   | 0.90 (0.39,2.09)   |
| PR                          | Positive | 0.50 (0.17,1.48)   | 0.54 (0.22,1.28)   | 0.50 (0.28,0.90)   | 0.49 (0.21,1.14)   |
| HER2                        | Positive | 0.58 (0.19,1.75)   | 0.68 (0.32,1.46)   | 0.40 (0.13,1.23)   | 0.52 (0.23,1.17)   |

## D Additional notes on “exact” imputation

As discussed in the main paper, we would like to impute missing values for each  $X_j$  iteratively within a chained equations imputation algorithm. Under *Assumptions 1-2*, we want to impute  $X_j$  from a distribution proportional to the following

$$f(X_j|X_{(-j)}, R) \propto f(X_j|X_{(-j)}) \prod_{k \neq j} f(R_k|X_j, X_{(-j)}).$$

**Categorical  $X_j$ :** When  $X_j$  is a categorical variable, we can express the exact probability mass function from the above equation as follows:

$$P(X_j = x|X_{(-j)}, R) = \frac{P(X_j = x|X_{(-j)}) \prod_{k \neq j} f(R_k|X_j = x, X_{(-j)})}{\sum_d P(X_j = d|X_{(-j)}) \prod_{k \neq j} f(R_k|X_j = d, X_{(-j)})}.$$

Defining  $PR_j(x) = P(R_j = 1|X_j = x, X_{(-j)})$ , we can express this probability mass function as

$$\frac{P(X_j = x|X_{(-j)}) \prod_{k \neq j} PR_k(x)^{R_k} [1 - PR_k(x)]^{1-R_k}}{\sum_d P(X_j = d|X_{(-j)}) \prod_{k \neq j} PR_k(d)^{R_k} [1 - PR_k(d)]^{1-R_k}}. \quad (\text{Eq. S1})$$

This probability is a function of the assumed model for  $X_j|X_{(-j)}$  and the missingness models for  $X_{(-j)}$ . We note that the distributions expressed in [Eq. S1](#) are obtained after having integrated out the corresponding parameters. We approximate a draw from [Eq. S1](#) by (1) drawing values for the parameter related to the  $X_j|X_{(-j)}$  distribution, (2) drawing parameters related to the missingness models  $f(R_k|X_j = x, X_{(-j)})$  for all  $k \neq j$ , and (3) drawing missing values for  $X_j$  from the probability mass function in [Eq. S1](#) with distributions evaluated at these drawn parameter values. One convenient strategy for drawing these parameters is to fit each of the target models to a bootstrap sample of the most recently imputed data. This may be all of the most recent imputed data or using the subset of patients with  $X_j$  observed.

**Continuous  $X_j$ :** When  $X_j$  is a continuous variable, the full form of the exact imputation distribution in [Eq. 1](#) is only known up to proportionality. Drawing from this distribution, therefore, requires more sophisticated strategies. Many strategies exist for drawing from a distribution known only up to proportionality, and we consider one such approach: rejection sampling.

Rejection sampling provides a strategy for obtaining an approximate draw from complicated distribution  $f(x)$  by drawing from a simpler distribution  $g(x)$ . In particular, suppose we can find distribution  $g(x)$  and scalar  $M \geq 1$  such that  $f(x) \leq Mg(x)$  for all  $x$ . Then, we can approximate a draw from  $f(x)$  by obtaining a candidate draw  $x^*$  from  $g(x)$  and accepting the candidate draw as the imputed value if  $U \leq f(x^*)/Mg(x^*)$  where random variable  $U$  is drawn from a uniform(0,1) distribution. We continue drawing candidates until one is accepted. For our problem, we define

$$f(x) = \frac{1}{C} f(X_j = x|X_{(-j)}) \prod_{k \neq j} f(R_k|X_j = x, X_{(-j)}) \quad (\text{Eq. S2})$$

and

$$g(x) = f(X_j = x|X_{(-j)})$$

where constant  $C$  is the proportionality constant such that the distribution integrates to 1. Using that  $\prod_{k \neq j} f(R_k|X_j = x, X_{(-j)}) \leq 1$ , we have that  $f(x) \leq \frac{1}{C}g(x)$ . This results in the following acceptance criterion:

$$\text{Accept } x^* \text{ if } U \leq \prod_{k \neq j} f(R_k|X_j = x^*, X_{(-j)}) = \prod_{k \neq j} PR_k(x^*)^{R_k} [1 - PR_k(x^*)]^{1-R_k}$$

When the missingness probabilities are not too large, this can result in a fairly efficient sampling strategy. As in the categorical case, all of these distributions involve implicit integration over the unknown model parameters, and we will draw from  $g(x)$  and evaluate  $\prod_{k \neq j} f(R_k | X_j = x, X_{(-j)})$  using drawn values of the corresponding model parameters.

## References

- [1] Ian R White, Rhian Daniel, and Patrick Royston. Avoiding bias due to perfect prediction in multiple imputation of incomplete categorical variables. *Computational Statistics and Data Analysis*, 54(4):2267–2275, 2010.
